# Supplementary material for: Tunneling study in granular aluminum near the Mott metal-to-insulator transition
Source: arXiv:2101.04994 source file (2021-07-29)
Supplement: Supplementary file 1 [file Supplemental_Material.pdf]

# Supplemental material for: Tunneling superconducting gap in granular aluminum at a BCS to BEC crossover near a Mott transition

## I. THZ SPECTROSCOPY

The data analysis of the raw data, i.e. the complex transmission $\hat{t} = |t|e^{i\phi_t}$ was done similarly as in previous work [1], in which there is a full description of the data analysis. The real part of the conductivity is shown in Fig. 1, along the Mattis-Bardeen [2] (MB) fits from which we extract twice the SC gap $\Omega$ value, marked by the minimum in $\sigma_1$. Most of the data follow the theory very well, except the sample with 6220 $\mu\Omega\, cm$ which shows a deviation from the fit around $4\Omega$, the origin of this deviation is not clear and is beyond the scope of this work.

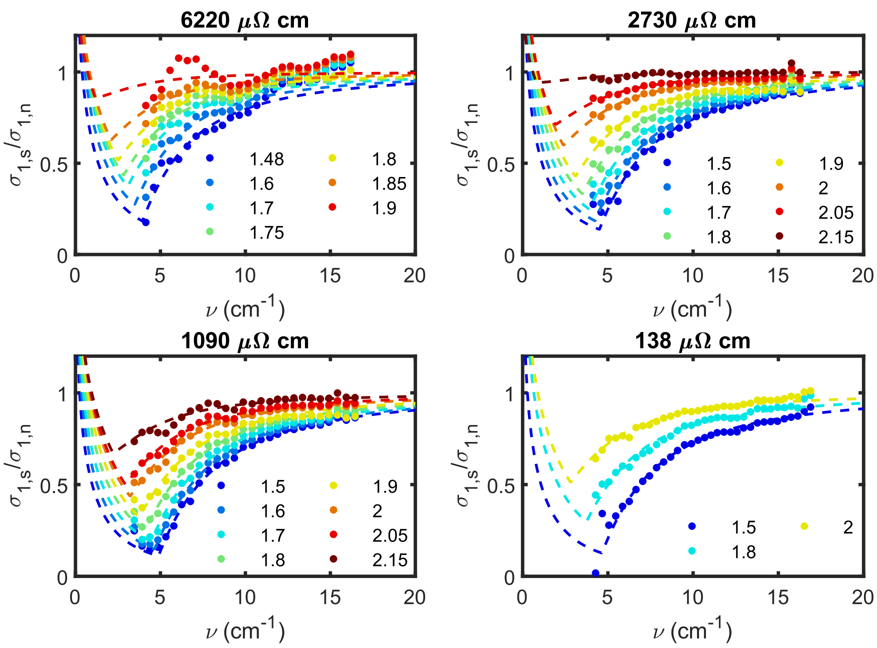


Figure S 1: Real part of the conductivity of all samples, normalized by the normal state value at $4.2\,$K. Dashed lines are fits to MB theory. The legend corresponds to the temperature at which the data was taken.

Next, we fit the obtained $\Omega(T)$ for each sample to the well known BCS gap equation [3], allowing us to obtain $\Omega_0$. The fits of $\Omega(T)$, along the resistive transition of the samples, are shown in Fig. 2.

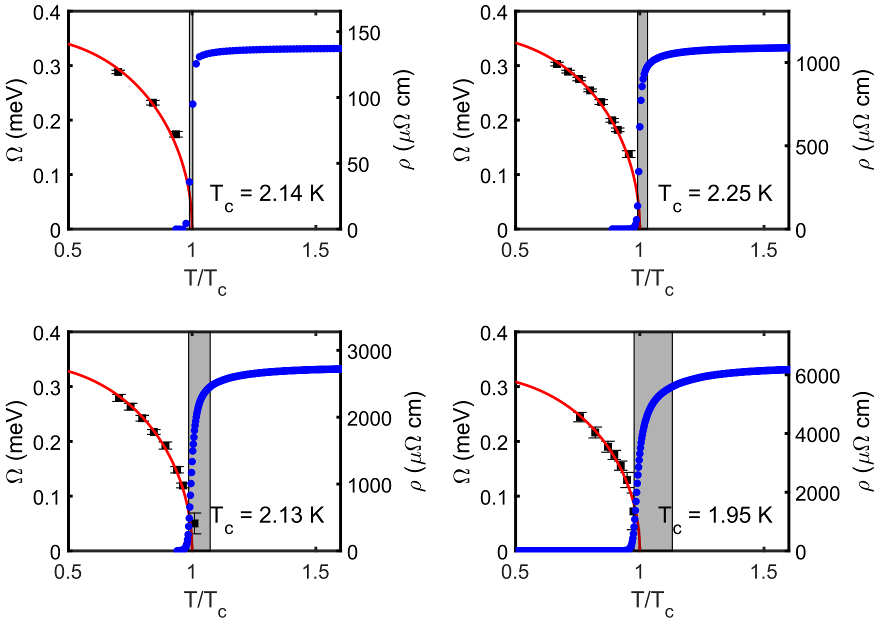


Figure S 2: Real part of the conductivity of all samples, normalized by the normal state value at $4.2\,\mathrm{K}$. Dashed lines are fits to MB theory. The error bars on $\Omega$ reflect the uncertainty in the MB fit of $\sigma_1(\omega)$.

## II. TUNNELING - DATA ANALYSIS AND ADDITIONAL FIGURES

### A. Data analysis

For samples measured down to about 1.5 K, we first fit the dI/dV spectrum to Eq. 1 in the main text for each temperature up to $T_c$. This procedure yields the temperature dependence of $\Gamma$ and $\Delta$. We extract $\Delta(T=0)=\Delta_0$ by fitting $\Delta(T)$ to the BCS gap equation [3] and we take $\Gamma$ as the measured value at the lowest temperature, which can be seen in Figs. 4 and 5 along the $\rho(T)$ curve. For samples measured down to 400 or 20 mK we take the values of $\Gamma$ and $\Delta$ directly as obtained from fitting to Eq. 1 in the main text. Representative differential conductance data for several samples, measured down to ~1.6-1.8 K, is shown in Fig. 3, along with the fit to Eq. 1 in the main text. The fitting for all studied samples has been limited to $\pm$ 1 meV.

An exception from the above was made for the sample having a resistivity of $65670\,\mu\Omega\,\mathrm{cm}$ and for the sample having a resistivity of $4134\,\mu\Omega\,\mathrm{cm}$ at temperatures close to $T_c$. As can be seen in Fig. 6(b), above the gap the differential conductance increases rapidly with voltage. To correctly obtain the superconducting DOS without the normal state influence, we fitted the data above 1.5 mV to the form $dI/dV = a + b\sqrt{|V|}$ and then divided by it the measured dI/dV for all measured voltages. We then fitted the resulted normalized differential conductance to Eq. 1 in the main text.

### B. Analysis of the magnetic field dependence

The field dependent data for a very high resistivity samples is shown in Figs. 7 and 8. To fit the data, we have used Eq. 1 in the main text with constant Al DOS for magnetic fields above 0.1 T (N-I-S junction) and a Dynes form of the Al DOS for the zero field data (S-I-S junction). In zero field, where the Al counter electrode is superconducting, sharp peaks corresponding to the sum of the gaps $\Delta_{\mathrm{Al}}+\Delta_{\mathrm{grAl}}$ are clearly observed in the dI/dV spectrum. The enhanced gap value of the Al electrode of about 0.24-0.26 meV is consistent with an increased critical temperature due to some release of oxygen during the deposition from the alumina coated Mb boat [4].

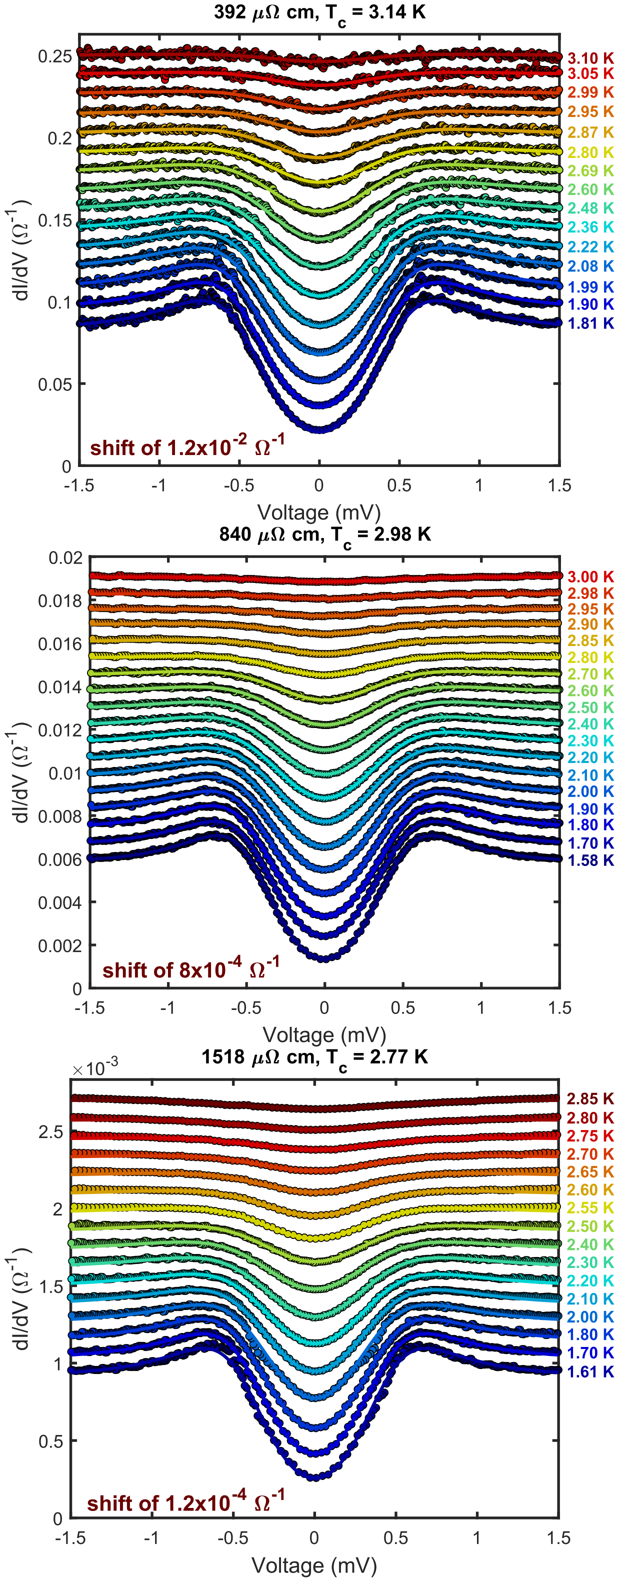


Figure S 3: Differential conductance spectrum at various temperatures for selected samples along the phase diagram, shifted for clarity. The thick lines are a fit to Eq. 1 in the main text. The inset of each figure shows the temperature dependence of $\Delta$ and $\Gamma$, along a fit to the BCS gap equation. The error bars on $\Delta$ and $\Gamma$ reflect the uncertainty in the Dynes fit of the differential conductance.

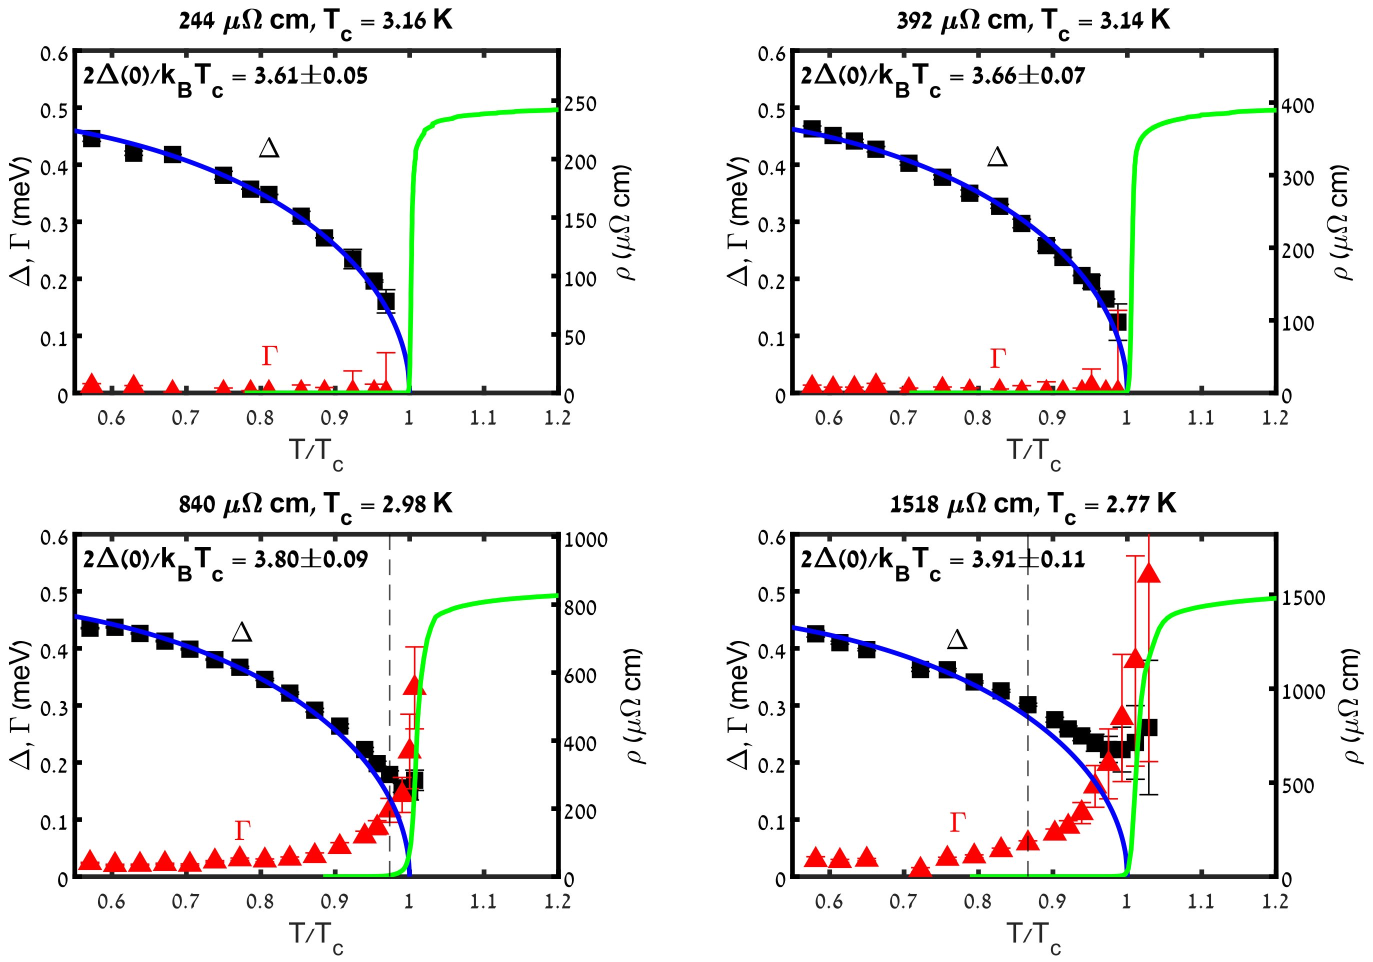


Figure S 4: Temperature dependence of $\Delta$ and $\Gamma$, along a fit to the BCS gap equation (blue line) and $\rho(T)$ (green line). The error bars on $\Delta$ and $\Gamma$ reflect the uncertainty in the Dynes fit of the differential conductance. The dashed vertical line marks the temperature which below it we fit the data points to the BCS equation, in order to avoid overestimation of the gap at low temperatures.

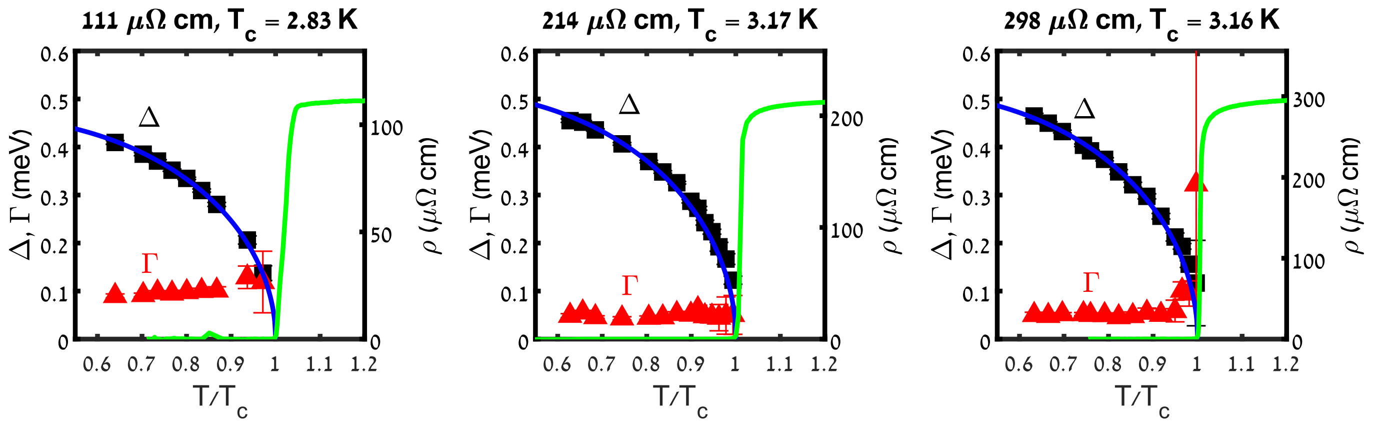


Figure S 5: Discarded samples data, shwoing the temperature dependence of $\Delta$ and $\Gamma$, along a fit to the BCS gap equation (blue line) and $\rho(T)$ (green line). The error bars on $\Delta$ and $\Gamma$ reflect the uncertainty in the Dynes fit of the differential conductance. Note how the value of $\Gamma$ is roughly temperature independent, indicating poor barrier quality.

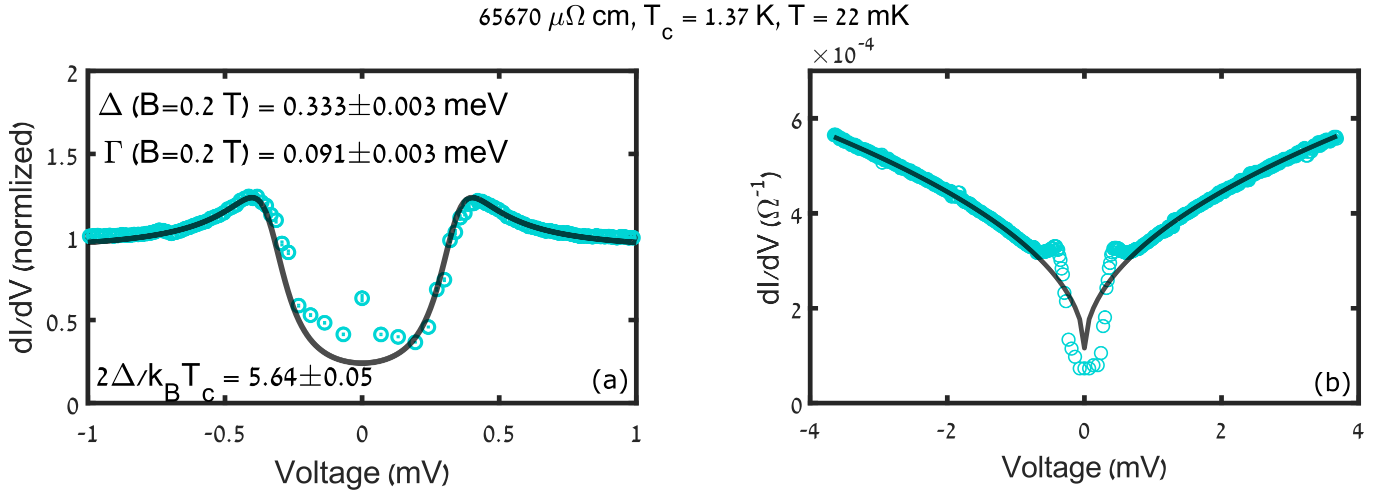


Figure S 6: Differential conductance data of the highest resistivity sample studied. Taken at 22 mK and 0.2 T magnetic field. (a) The normalized data along a fit to Eq. 1 in the main text. (b) The raw data along a fit to the form $dI/dV \propto \sqrt{|V|}$. Note that the conductance is strongly depressed over an energy scale that is compatible with the predictions of DMFT theory.

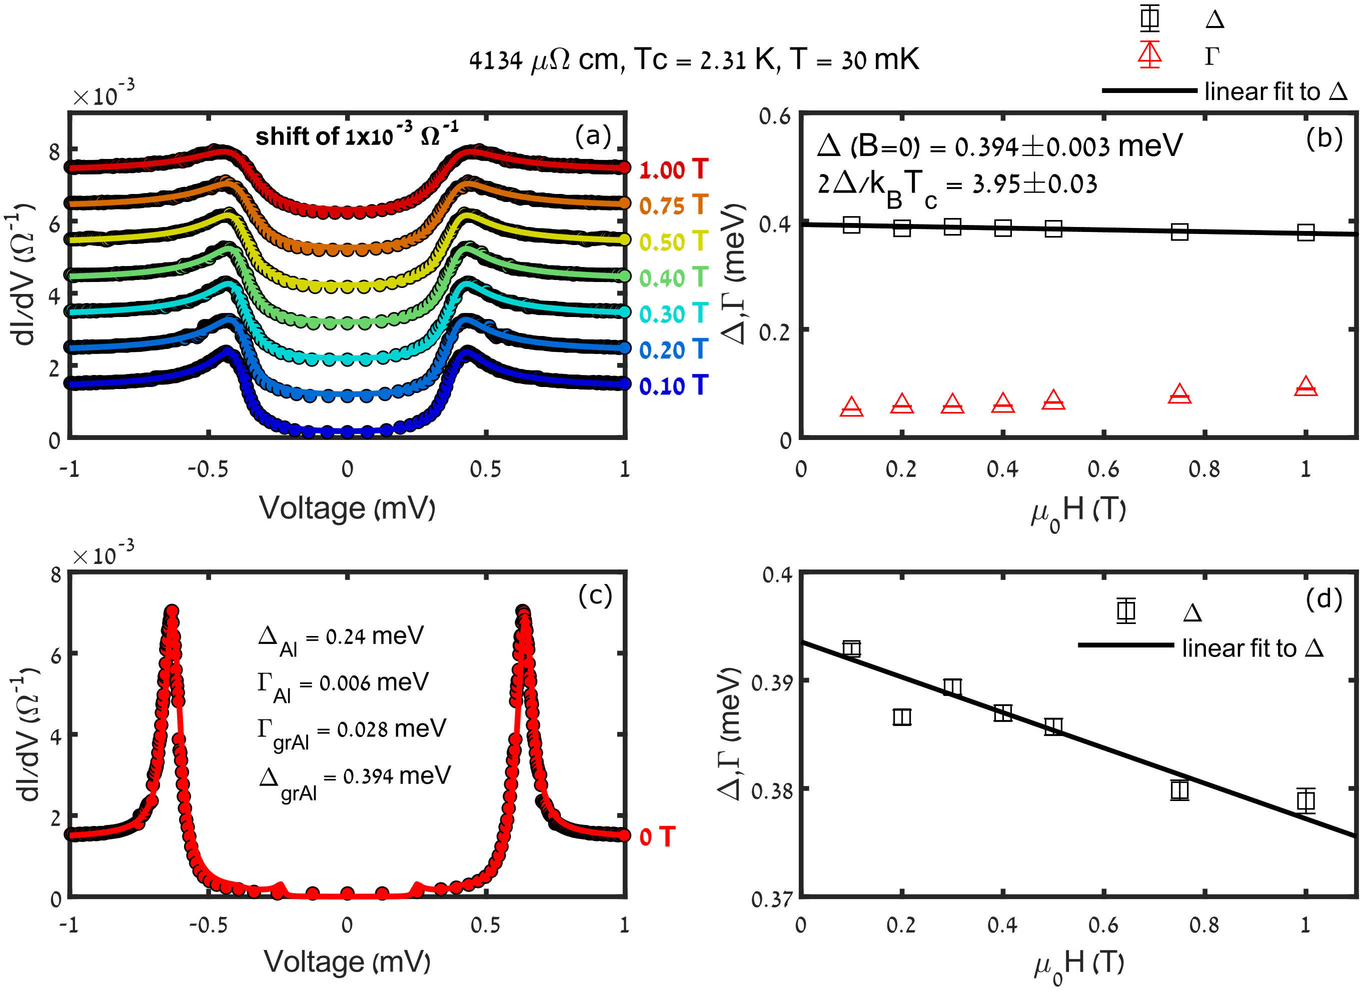


Figure S 7: Magnetic field analysis for sample having a resistivity of 4134 $\mu\Omega$ cm. (a) dI/dV data (shifted for clarity) at various magnetic fields up to 1 T, the circles are the data points and the lines are fits to Eq. 1 in the main text. The broadening of the peaks with increasing field is clearly observed. (b) The values of $\Gamma$ and $\Delta$ as obtained from the fits, along a linear fit to $\Delta$, used to extrapolate its zero field value. (c) Zero field data. The circles are the data points and the red line is a fit to Eq. 1 in the main text for a SIS junction, where we used a Dynes form of the density of states for both superconducting electrodes. (d) Same data as in (b) but zoomed in for clarity.

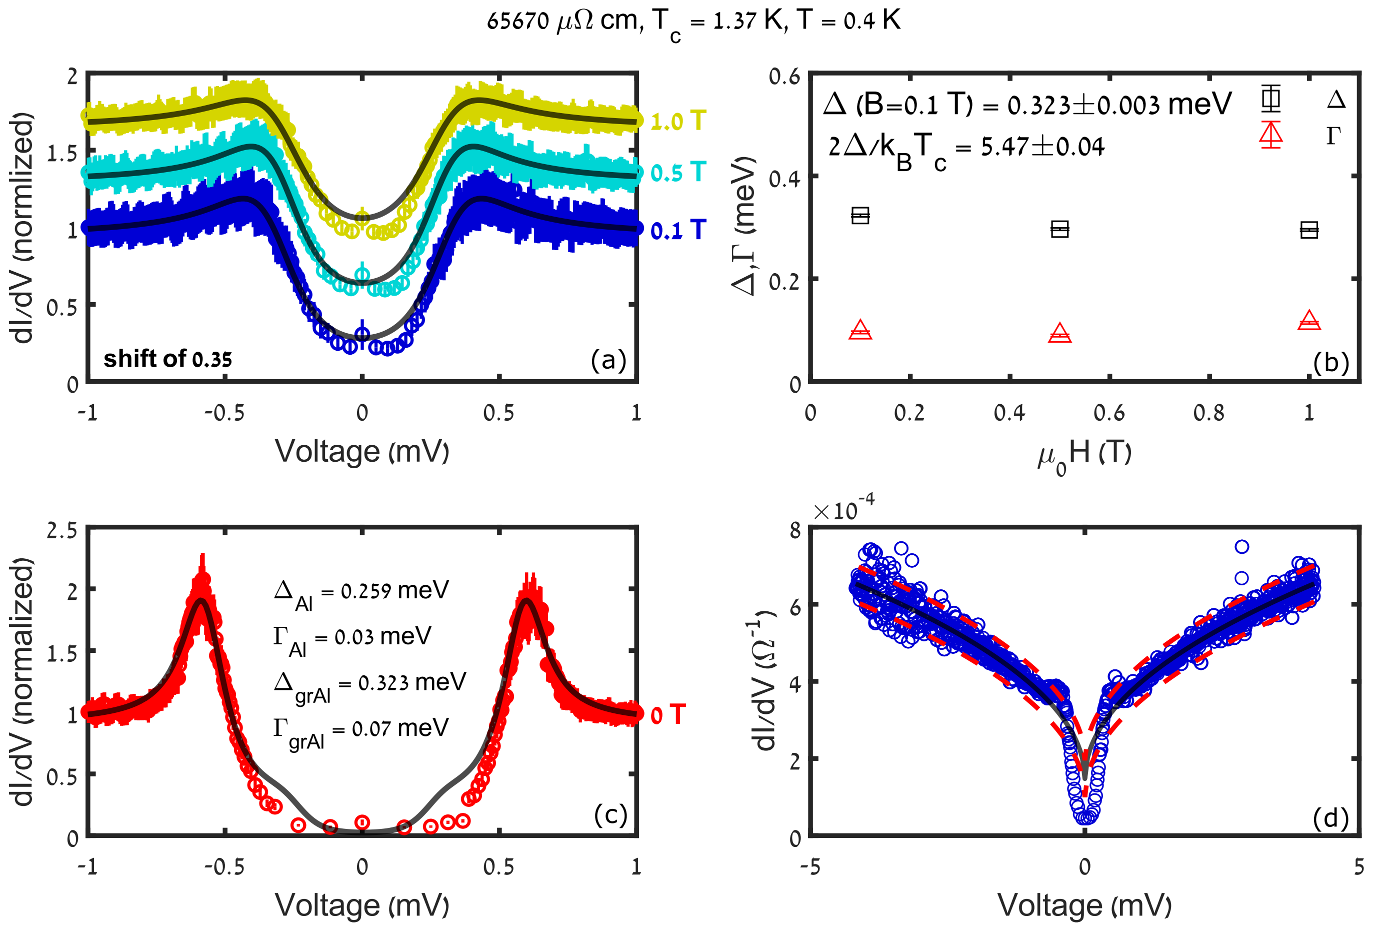


Figure S 8: Magnetic field analysis for sample having a resistivity of 65,670 $\mu\Omega$ cm. (a) normalized dI/dV data (shifted for clarity) at various magnetic fields up to 1 T, the circles are the data points and the lines are fits to Eq. 1 in the main text. The error bars have been determined by the 95% confidence interval of the $dI/dV \propto \sqrt{|V|}$ fit above 1.5 mV, used to divide the data for all voltages. (b) The values of $\Gamma$ and $\Delta$ as obtained from the fits. (c) Zero field data. The circles are the data points and the red line is a fit to Eq. 1 in the main text for a SIS junction, where we used a Dynes form of the density of states for both superconducting electrodes. (d) High voltage data at 0.1 T along the $dI/dV \propto \sqrt{|V|}$ fit. The dashed lines are the 95% confidence interval predicted bounds.

[1] A. G. Moshe, E. Farber, and G. Deutscher, Phys. Rev. B **99**, 224503 (2019).
[2] D. C. Mattis and J. Bardeen, PR **111**, 412 (1958).
[3] J. Bardeen, L. N. Cooper, and J. R. Schrieffer, Phys. Rev. **108**, 1175 (1957).
[4] R. W. Cohen and B. Abeles, Phys. Rev. **168**, 444 (1968).
